# Supplementary material for: How Does Generative Retrieval Scale to Millions of Passages?
Source: arXiv:2305.11841 source file (2023-05-19)
Supplement: Supplementary file 1 [file appendix.tex]

\appendix
\section{Appendix}
\subsection{Improving Synthetic Query Generation}

From Figure~\ref{fig:jaccard_mrr}, it is clear that with more exposure to synthetic queries, the model generally demonstrates higher effectiveness across all subsets.
This further fortifies the significance of better and more diverse synthetic query generation in the generative information retrieval task.
In this section, we empirically investigate three question generation boosting, namely,
improving diversify and faithfulness, and, training the generation model
on in-domain training data. 

\paragraph{More diversified synthetic questions helps.}
We simply tuning the decoding hyper-parameter by increasing the beam size to $100$ when
continuing using top-k sampling ($k=10$, $temperature=1.0$). The results are summarised in the
top block in Table~\ref{table:v1:passage_n_queries}. 
Increasing beam size from 40 to 100, the unique questions per passage are more than doubled, increased from
26 to 58, thus introducing more diversified synthetic questions. 
This actually brings in considerable boost, increasing MRR@10 from 79.6 to 82.4, 
closing the gap relative to GTR-base (83.2) on MSMarco100K. 
% We further do the same experiments on MSMarco1M and MSMarcoFULL, and the results are in Table~\ref{}.

\paragraph{Filtering the synthetic questions with the state-of-the-art cross-attention re-ranker does not help.}
Recent studies show advances in utilizing cross encoders to refine the generated query set of incoherent, unspecific queries~\citet{d2q-less-more} to improve the use of D2Q.
Likewise, we leverage a RankT5-XL~\cite{zhuang22rankt5} model, to score (generated query, passage) pairs before filtering out those generated queries that give a low ranking score.
The threshold is such that we filter out $x\%$ of the queries to make the query set more relevant, coherent and hallucination-free.
This can be considered both as a global threshold, as in we filter out $x\%$ of all queries in the generated query set or a local threshold where we filter out $x\%$ of queries belonging to a particular identifier. The results are included in the lower block in Table~\ref{table:v1:passage_n_queries}. It can be seen that, the filtering does not help to boost the model. 

\paragraph{Use of in-domain question generation model helps.}
As mentioned in Section~\ref{sec.methods}, 
we reuse the D2Q from NCI code repository, which are generated using a question generation model
trained on MSMarco dataset~\cite{nogueira2019doc2query}.
Instead, we fine-tune a T5-base model on DPR~\cite{karpukhin2020dense} dataset for 50K steps with batch size 512, and generate synthetic questions for NQ100K and TriviaQA using the same parameters as in~\cite{nogueira2019doc2query}. The results are summarised in Table~\ref{table:v1:nci_small_scale} (row (7)). It can be seen that, the use of in-domain D2Q could considerably boost the results (except for semantic IDs on TriviaQA) considerably.

% \paragraph{F3. Convert document/passage retrieval to question retrieval.}
% Orthogonal to above assumptions,
% another possibility is that D2Q actually converts the problem from document/passage retrieval to
% question retrieval~\cite{}.
% To examine this, we study the correlation between the highest similarity of a test query/question relative to all generated questions, and the retrieval performance. Specifically,
% for each question/query from evaluation dataset, 
% we compute its cosine similarity with respect to all generated questions and record the maximum similarity;
% in the meantime, we correlate this similarity with its retrieval quality. 
% Furthermore, we investigate the use of our model on Quora Duplicate-Question dataset and summarise the results in Table~\ref{}. 

% Table~\ref{table:v1:passage_n_queries}

Given the generation-only training effectiveness of NQ showing higher effectiveness than MS-100K despite similar coverage, we further investigate why this might.
We begin with noticing that NQ has on average 3 queries per documents in the training query set as opposed to MS MARCO with 1 query.
To verify if this is the root cause, we filter the NQ training query set to include only 1 query for each passage and find that the effectiveness drops considerably, with a Hits@1 of 3.
% https://tensorboard.corp.google.com/experiment/7604697821758015566/?darkMode=true&forceSVG=true#timeseries
Hence, it seems critical to modeling effectiveness that there is multiple queries for each passage, given that a single exposure might lead the model to attributing the task to simple text mapping to identifiers, in which case, this could be simplified as simply seeing the mapping of the test query.
